# Supplementary material for: Lie Algebraic Similarity Transformed Hamiltonians for Lattice Model Systems
Source: arXiv:1409.2203 ancillary file (2014-11-10)
Supplement: Supplementary file 1 [file Supplemental_Material.pdf]

# Suplemental Information for "Lie Algebraic Similarity Transformed Hamiltonians for Lattice Model Systems"

Jacob M. Wahlen-Strothman,[1] Carlos A. Jiménez-Hoyos,[2] Thomas M. Henderson,[1,2] and Gustavo E. Scuseria[1,2]

[1]*Department of Physics and Astronomy, Rice University, Houston, Texas 77005, USA*
[2]*Department of Chemistry, Rice University, Houston, Texas 77005, USA*

(Dated: November 9, 2014)

## CORRELATOR HAUSDORFF SERIES

We wish to show that

$$e^{-J} c^\dagger_{k\sigma} e^J = e^{-J_{k\sigma}} c^\dagger_{k\sigma}, \tag{1}$$

with the definition

$$J_{k\sigma} = \sum_{i\sigma'} \alpha_{k\sigma,i\sigma'} n_{i\sigma'}. \tag{2}$$

can be summed exactly. Expand the commutator series

$$e^{-J} c^\dagger_{k\sigma} e^J = c^\dagger_{p\sigma} + \left[c^\dagger_{k\sigma}, J\right] + \frac{1}{2}\left[\left[c^\dagger_{k\sigma}, J\right], J\right] + ... \tag{3}$$

The first commutator is

$$\left[c^\dagger_{k\sigma}, J\right] = \frac{1}{2}\sum_{j\sigma'',i\sigma'} \alpha_{j\sigma'',i\sigma'}\left[c^\dagger_{k\sigma}, n_{i\sigma'} n_{j\sigma''}\right] \tag{4}$$

$$= -\sum_{i\sigma'} \alpha_{k\sigma,i\sigma'} n_{i\sigma'} c^\dagger_{k\sigma}$$

$$= -J_{k\sigma} c^\dagger_{k\sigma}. \tag{5}$$

The second commutator is

$$\left[\left[c^\dagger_{p\sigma}, J\right], J\right] = -J_{k\sigma}\left[c^\dagger_{k\sigma}, J\right] \tag{6}$$

$$= J^2_{k\sigma} c^\dagger_{k\sigma}$$

because

$$\left[J_{k\sigma}, J\right] = 0. \tag{7}$$

From here, the main result follows immediately.

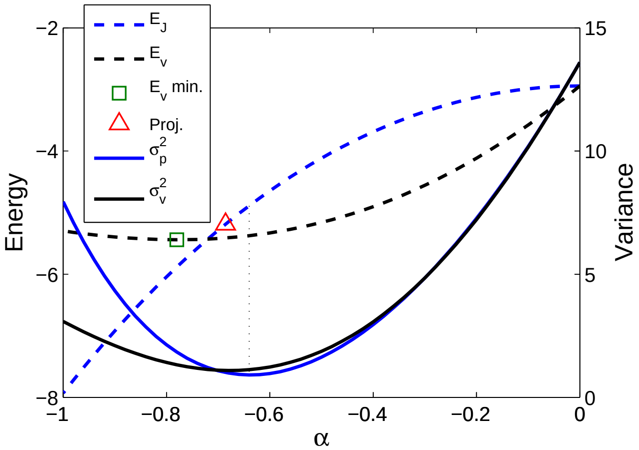


FIG. 1. Transformed and variational energies and variances for periodic half-filled, 10-site Hubbard with $U = 4$ using the Gutzwiller factor $J = \sum_i \alpha n_{i\uparrow} n_{i\downarrow}$ on an RHF reference.

## PROJECTIVE AND VARIANCE OPTIMIZATION

To illustrate the relation between the transformed Hamiltonian $\overline{H} = e^{-J} H e^J$ and the correlated wavefunction $e^J|\Phi\rangle$, we compare the variational and transformed energies and the respective energy variances (S. Tsuneyuki, Prog. Theor. Phys. Suppl. **176**, 134 (2008))

$$\sigma^2_J = \langle \overline{H}^\dagger \overline{H}\rangle - |\langle \overline{H}\rangle|^2 \tag{8}$$

$$\sigma^2_v = \frac{\langle e^J H^2 e^J\rangle}{\langle e^{2J}\rangle} - \left|\frac{\langle e^J H e^J\rangle}{\langle e^{2J}\rangle}\right|^2, \tag{9}$$

for the Gutzwiller factor in Fig. 1, as the variance is a direct measure of the quality of the wavefunction. The transformed energy, $E_J = \langle \overline{H}\rangle$, and the hermitian expectation value $E_v = \langle e^J H e^J\rangle / \langle e^{2J}\rangle$, cross near the value of $\alpha$ which minimizes $E_v$ and thus the latter can be approximated finding an optimal $\alpha$. Both the minimum of $\sigma^2_J$ indicated by the dotted line and the solution to the projective equations produce values for $\alpha$ very near this crossing. The projective equations are less expensive and easier to converge in our experience.

## RESULTS FOR 1D SYSTEMS

Correlation energies based on RHF at half-filling are presented in Fig. 2. The method is most accurate for small $U$ and small systems, but a large portion of the correlation energy is still recovered at larger $U$.

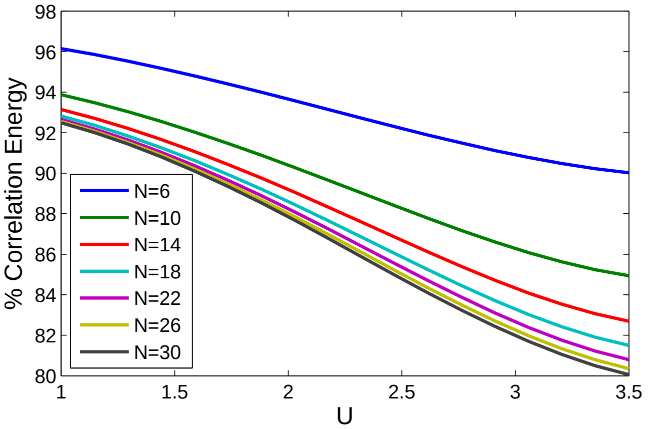


FIG. 2. Correlation energy captured by Gutzwiller, spin-spin, and density-density correlators as a function of interaction for different periodic systems at half-filling on an RHF reference.

## RESULTS FOR 4X4 LATTICES

Results for various fillings and interaction strengths in periodic $4 \times 4$ Hubbard lattices are presented below with both RHF and UHF references. The correlators are capable of recovering a large portion of the correlation energy over all fillings and values of $U$.

| $N_o$ | $U$ | $E_{RHF}$ | $E_{UHF}$ | $E_{RJ}$ | $E_{UJ}$ | $E_{ED}$ | $\%E_c(RJ)$ | $\%E_c(UJ)$ |
|---|---|---|---|---|---|---|---|---|
| 4 | 4 | -0.6875 | -0.7053 | -0.7120 | -0.7194 | -0.7206 | 73.93 | 96.33 |
| 4 | 8 | -0.6250 | -0.6663 | -0.6962 | -0.7048 | -0.7076 | 86.19 | 96.55 |
| 4 | 12 | -0.5625 | -0.6345 | -0.6878 | -0.6959 | -0.7003 | 90.94 | 96.84 |
| 6 | 4 | -0.8594 | -0.9000 | -0.9105 | -0.9274 | -0.9460 | 58.97 | 78.55 |
| 6 | 8 | -0.7187 | -0.8240 | -0.8723 | -0.8927 | -0.9202 | 76.24 | 86.36 |
| 6 | 12 | -0.5781 | -0.7730 | -0.8526 | -0.8733 | -0.9061 | 83.69 | 89.99 |
| 8 | 4 | -1.0000 | -1.0249 | -1.0811 | -1.0885 | -1.0959 | 84.55 | 92.24 |
| 8 | 8 | -0.7500 | -0.8469 | -1.0052 | -1.0031 | -1.0288 | 91.52 | 90.77 |
| 8 | 12 | -0.5000 | -0.7572 | -0.9767 | -0.9347 | -0.9941 | 96.47 | 87.97 |
| 10 | 4 | -1.1094 | -1.1094 | -1.2162 | -1.2162 | -1.2238 | 93.35 | 93.35 |
| 10 | 8 | -0.7187 | -0.8490 | -1.0678 | -1.0157 | -1.0944 | 92.93 | 79.06 |
| 10 | 12 | -0.3281 | -0.7393 | -0.9787 | -0.9284 | -1.0284 | 92.91 | 85.72 |
| 12 | 4 | -0.9375 | -0.9861 | -1.0837 | -1.0898 | -1.1080 | 85.75 | 89.30 |
| 12 | 8 | -0.3750 | -0.7091 | -0.8694 | -0.8483 | -0.9328 | 88.63 | 84.85 |
| 12 | 12 | 0.1875 | -0.5967 | -0.8508 | -0.7491 | -0.8512 | 99.96 | 90.17 |
| 14 | 4 | -0.7344 | -0.8808 | -0.9018 | -0.9595 | -0.9840 | 67.06 | 90.18 |
| 14 | 8 | 0.0313 | -0.5921 | -0.5354 | -0.6691 | -0.7418 | 73.30 | 90.60 |
| 14 | 12 | 0.7969 | -0.4744 | -0.3158 | -0.5488 | -0.6282 | 78.08 | 94.43 |
| 16 | 4 | -0.5000 | -0.7854 | -0.6931 | -0.8270 | -0.8514 | 54.94 | 93.06 |
| 16 | 8 | 0.5000 | -0.4619 | -0.2235 | -0.4873 | -0.5293 | 70.29 | 95.92 |
| 16 | 12 | 1.5000 | -0.3208 | -0.0447 | -0.3326 | -0.3745 | 82.41 | 97.76 |

TABLE I. Correlated energies for $4 \times 4$ Hubbard lattices on RHF ($E_{RJ}$) and UHF ($E_{UJ}$) references and the portion of the correlation energy recovered ($E_c$) with $Sz = 0$, exact energies ($E_{ED}$) taken from: H. Shi, S. Zhang, Phys. Rev. B **88**, 125132 (2013). $E_{UJ}$ includes spin-density correlators ($S_i^z N_j$).
